# Supplementary material for: DeltaDock: A Unified Framework for Accurate, Efficient, and Physically Reliable Molecular Docking
Source: arXiv:2410.11224 source file (2024-10-16)
Supplement: Supplementary file 1 [file 7_appendix_rebuttal.tex]

\appendix
\clearpage
\makeatletter 
\makeatother
\setcounter{figure}{0}
\setcounter{table}{0}
\setcounter{page}{1}
\renewcommand{\appendixname}{Appendix~\Alph{section}}

\section{Appendix PDF for Rebuttal}
This section presents additional experimental results to further evaluate the performance of \modelname. We include the recent blind docking method FABind+ as a baseline for comparison.
Our results demonstrate that \modelname consistently achieves a higher docking success rate than FABind+, particularly on unseen datasets. Furthermore, when analyzing performance on the PoseBusters dataset, considering physical validity, FABind+ experiences a significant drop in performance, whereas \modelname maintains its effectiveness.


 \begin{figure}[h]
 \centering
  \includegraphics[width=0.93\linewidth]{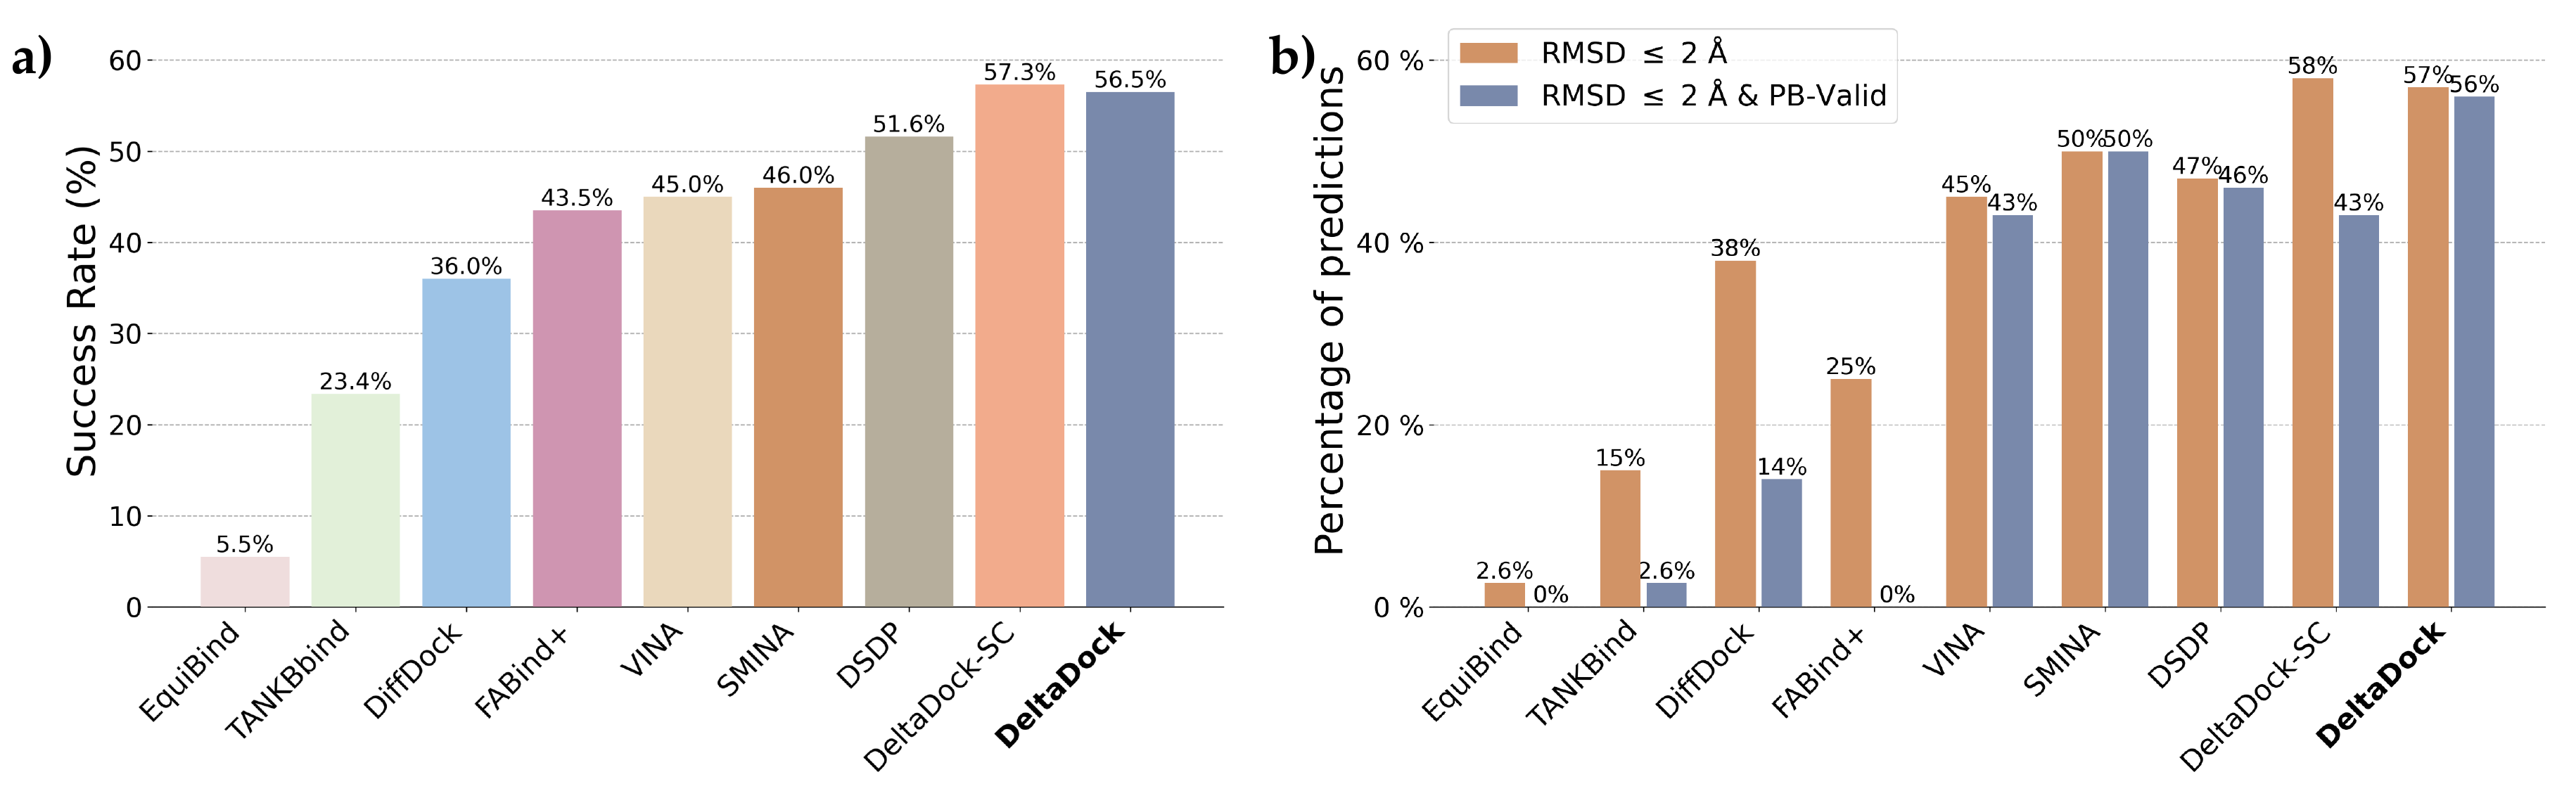}
  \vspace{-0.1in}
  \caption{Site-specific docking performance.
  (a) Overall Performance of different methods on the PDBbind test set.
  (b) Overall performance of different methods on the PoseBusters dataset.}
 \end{figure}

\vspace{-0.1in}

 \begin{table*}[h]
 \centering
 \caption{Blind docking performance on the PDBbind dataset.  The best results are {\bf bold}, and the second best results are \underline{underlined}.}
 \label{tbl:blind_docking_test_set}
\begin{adjustbox}{width=1\textwidth}
\begin{threeparttable}
\begin{tabular}{lccccccccccccc}
\toprule
\multirow{3}{*}{Method} &
\multirow{2}{*}{Time average} & \multicolumn{6}{c}{Ligand RMSD} & \multicolumn{6}{c}{Centroid Distance}\\
% \cline{3-14}
& & \multicolumn{4}{c}{Percentiles} & \multicolumn{2}{c}{ \% below Threshold}  & \multicolumn{4}{c}{Percentiles} & \multicolumn{2}{c}{ \% below Threshold} \\
% \cline{2-14}
& Seconds & 25\% & 50\% & 75\% & mean & 2\AA  & 5\AA & 25\% & 50\% & 75\% & mean & 2\AA & 5\AA \\
\midrule
QVINA-W
& 49 & 2.5 & 7.7 & 23.7 & 13.6 & 20.9 & 40.2 & 0.9 & 3.7 & 22.9 & 11.9 & 41.0 & 54.6 \\
GNINA
& 393 & 2.8 & 8.7 & 21.2 & 13.3 & 21.2 & 37.1 & 1.0 & 4.5 & 21.2 & 11.5 & 36.0 & 52.0 \\
VINA
& 119 & 3.7 & 6.8 & 14.6 & 10.1 & 10.3 & 36.2 & 1.5 & 4.1 & 13.3 & 8.2 & 32.3 & 55.2 \\ 
SMINA
& 146 & 3.8 & 8.1 & 13.5 & 12.1 & 13.5 & 33.9 & 1.3 & 3.7 & 16.2 & 9.8 & 38.0 & 55.9 \\
GLIDE
& 1405 & 2.6 & 9.3 & 21.8 & 16.2 & 21.8 & 33.6 & 0.8 & 5.6 & 26.9 & 14.4 & 36.1 & 48.7 \\
DSDP 
& 1.22* & 1.0 & 3.0 & 7.9 & 7.2 & 42.4 & 59.8 & \textbf{0.3} & 1.0 & 4.8 & 4.9 & 60.3 & 75.8 \\ 
\midrule
EquiBind
& \underline{0.03*} & 3.8 & 6.2 & 10.3 & 8.2 & 5.5 & 39.1 & 1.3 & 2.6 & 7.4 & 5.6 & 40.0 & 67.5 \\
TANKBind
& 0.87* & 2.4 & 4.2 & 7.6 & 7.8 & 17.6 & 57.8 & 0.8 & 1.7 & 4.3 & 5.9 & 55.0 & 77.8 \\
DiffDock
& 80* & 1.5 & 3.5 & 7.4 & 7.4 & 36.0 & 61.7 & 0.5 & 1.2 & 3.3 & 5.4 & 62.9 & 80.2 \\
FABind
& 0.12* & 1.7 & 3.1 & 6.7 & 6.4 & 33.1 & 64.2 & 0.7 & 1.3 & 3.6 & 4.7 & 60.3 & 80.2 \\
FABind+
& 0.16* & 1.2 & 2.6 & \underline{5.8} & \underline{5.2} & 43.5 & \underline{71.1} & \underline{0.4} & 1.0 & 2.9 & \textbf{3.5} & 67.5& \underline{84.0} \\
FABind+(40)
& 6.4* & 1.2 & 2.4 & \textbf{5.3} & \textbf{5.1} & 43.8 & \textbf{73.3} & 0.5 & 1.0 & \textbf{2.6 }& \textbf{3.5} & \underline{69.1} & \textbf{86.2} \\
\midrule
\textbf{\modelname-SC}
&
2.58* & \underline{1.1} & \underline{2.3} & 6.2 & 5.7 & \textbf{47.9} & 68.0 & \underline{0.4} & \textbf{0.8} & \textbf{2.6} & 4.1 & \textbf{70.0} & 83.2  \\
\textbf{\modelname}
&
2.97* & \textbf{1.0} & \textbf{2.2} & 6.4 & 5.8 & \underline{47.4} & 66.9 & \textbf{0.3} & \underline{0.9} & 2.9 & 4.2 & 66.7 & 83.2  \\
\bottomrule
\end{tabular}
\begin{tablenotes}
 \item[1] The time of consumption is denoted with * if it corresponds to GPU time; in the absence of this symbol, the time pertains to CPU time.
\end{tablenotes}
\end{threeparttable}
\end{adjustbox}

\end{table*}

\vspace{-0.1in}

\begin{table*}[h]
\centering
 \caption{Blind docking performance for PDBbind unseen dataset.  The best results are {\bf bold}, and the second best results are \underline{underlined}.}
 
\label{tbl:blind_docking_unseen_set}
\begin{adjustbox}{width=1\textwidth}
\begin{threeparttable}
\begin{tabular}{lccccccccccccc}
\toprule
\multirow{3}{*}{Method}
& \multicolumn{6}{c}{Ligand RMSD} & \multicolumn{6}{c}{Centroid Distance}\\
% \cline{3-14}
& \multicolumn{4}{c}{Percentiles} & \multicolumn{2}{c}{ \% below Threshold}  & \multicolumn{4}{c}{Percentiles} & \multicolumn{2}{c}{ \% below Threshold} \\
% \midrule{3-6}
& 25\% & 50\% & 75\% & mean & 2\AA  & 5\AA & 25\% & 50\% & 75\% & mean & 2\AA & 5\AA \\
\midrule
QVINA-W
& 3.4 & 10.3 & 28.1 & 16.9 & 15.3 & 31.9 & 1.3 & 6.5 & 26.8 & 11.9 & 35.4 & 47.9 \\
GNINA
& 4.5 & 13.4 & 27.8 & 16.7 & 13.9 & 27.8 & 2.0 & 10.1 & 27.0 & 15.1 & 25.7 & 39.5 \\
VINA
& 5.0 & 9.6 & 19.0 & 12.8 & 7.8 & 25.5 & 2.2 & 6.1 & 17.8 & 10.9 & 24.1 & 41.8 \\
SMINA
& 4.8 & 10.9 & 26.0 & 15.7 & 9.0 & 25.7 & 1.6 & 6.5 & 25.7 & 13.6 & 29.9 & 41.7 \\
GLIDE
& 3.4 & 18.0 & 31.4 & 19.6 & 19.6 & 28.7 & 1.1 & 17.6 & 29.1 & 18.1 & 29.4 & 40.6 \\
DSDP
& 1.0 & 4.5 & 10.0 & 9.1 & 37.2 & 54.9 & \textbf{0.2} & 1.5 & 6.5 & 7.5 & 54.2 & 69.0 \\
\midrule
EQUIBIND
& 5.9 & 9.1 & 14.3 & 11.3 & 0.7 & 18.8 & 2.6 & 6.3 & 12.9 & 8.9 & 16.7 & 43.8 \\
TANKBind
& 3.0 & 4.9 & 8.7 & 9.3 & 4.9 & 52.1 & 1.3 & 2.3 & 4.4 & 7.2 & 41.5 & 76.1 \\
DiffDock
& 2.9 & 6.4 & 16.3 & 12.0 & 17.2 & 42.3 & 1.0 & 2.7 & 14.2 & 9.8 & 43.3 & 62.6 \\
FABind
& 2.2 & \underline{3.4} & 8.3 & 7.7 & 19.4 & 60.4 & 0.9 & 1.5 & 4.7 & 5.9 & 57.6 & 75.6 \\
FABind+
& 1.6 & \textbf{3.3} & 8.9 & 7.0 & 34.7 & \textbf{63.2} & \underline{0.5} & 1.5 & 4.2 & 5.1 & 58.3 & 77.1 \\
\midrule
\textbf{\modelname-SC}
& \underline{}{1.2} & 3.9 & \underline{7.8} & \textbf{5.7} & \textbf{40.8} & 60.5 & \underline{0.5} & \textbf{1.2} & \textbf{4.0} & \textbf{4.1} & \textbf{65.5} & \textbf{78.9} \\
\textbf{\modelname}
& \textbf{1.0} & 3.8 & \textbf{7.7} & \underline{5.8} & \textbf{40.8} & \underline{61.3} & \textbf{0.4} & \textbf{1.2} & \underline{4.1} & \underline{4.2} & \underline{60.6} & \textbf{78.9} \\
\bottomrule
\end{tabular}
\begin{tablenotes}
 \item[1] The time of consumption is denoted with * if it corresponds to GPU time; in the absence of this symbol, the time pertains to CPU time.
\end{tablenotes}
\end{threeparttable}
\end{adjustbox}

\end{table*}
